# Supplementary material for: Boosting Distributed Full-graph GNN Training with Asynchronous One-bit Communication
Source: arXiv:2303.01277 source file (2023-03-02)
Supplement: Supplementary file 1 [file 8_Appendix.tex]

%\newpage
\onecolumn
%-------------------------------------------------------------------------------
\section{Formulations}
%-------------------------------------------------------------------------------
\subsection{Table of Notations}
\begin{table}[ht]
    \centering
    \caption{Detailed information of datasets.}
    \vskip 0.1in
    \resizebox{0.5\linewidth}{!}{
        \begin{tabular}{@{}ccl@{}}
\toprule
\textbf{Notation}                                                                                                        & \textbf{Description}                              &  \\ \midrule
$B$                                                                                                                      & \multicolumn{1}{l}{Number   of quantization bins} &  \\
$D$                                                                                                                      & Model hidden size                                 &  \\
$\boldsymbol{H}^{(l)}$                                                                                                   & Embedding matrix of $l$-th layer                  &  \\
$\boldsymbol{W}^{(l)}$                                                                                                   & Weights of $l$-th layer                           &  \\
$\mathbf{B}^{(l)}()$                                                                                                     & Backward function of the $l$-th layer             &  \\
$\mathbf{C}\left(\boldsymbol{H}^{(l-1)},   \boldsymbol{W}^{(l)}\right),\mathbf{C}^{(l)}$                                 & Context of $l$-th layer                           &  \\
\multicolumn{1}{l}{$\hat{\mathbf{C}}\left(\boldsymbol{H}^{(l-1)},   \boldsymbol{W}^{(l)}\right),\hat{\mathbf{C}}^{(l)}$} & Quantized context of $l$-th layer                 &  \\
$\boldsymbol{J}^{(l)}$                                                                                                   & Feature gradients                                 &  \\
$\boldsymbol{G}^{(l)}$                                                                                                   & Weight gradients                                  &  \\
$\mathcal{L}$                                                                                                              & Loss of prediction and label                      &  \\ \bottomrule
\end{tabular}
            }
    \label{table_notations}
    \vskip 0.2in
\end{table}

\subsection{The Algorithm of \SysNameP}
\label{app_algop}
Section \ref{algo} presents the algorithm of \SysName in the forward and backward phases, respectively. Here we further provide the detailed algorithm of the pipelined version, \SysNameP. 

\textbf{Forward Propogation}. The forward phase of \SysNameP on each partition is outlined in Alg.\ref{pfw}. Most parts are the same as that in \SysNameS, except that the embedding communication is overlapped with the forward computation, as shown in line 14-21. Here we initialize the node embedding by concatenating the original features and zero vectors. At each layer, the forward computation starts in parallel with \textit{1-bit Module} and the communication of embeddings. Note that the transmitted embeddings in current epoch are prepared in the buffer for the next epoch, which could lead to stale embeddings.

\begin{algorithm}[ht]
    \caption{Forward phase of \SysNameP}
    \small
    \label{pfw} 
    \begin{algorithmic}[1]
        \INPUT Partition id $n$, subgraph $\mathcal{G}_n$, feature matrix $\boldsymbol{X}_n$, label $Y_n$, adjacency matrix $\boldsymbol{A}_n$, epoch number $T$, layer size $L$, local node set $V_n$, weights $\boldsymbol{W}^{(l-1)}$ 
        \STATE \textbf{Partition} $n=1,2,...,N$ in Parallel: 
        \STATE $\boldsymbol{H}^{(0)}_n=\left[\begin{matrix}\boldsymbol{X}_n & 0 \end{matrix}\right]^\top$ \COMMENT{Initialize node embeddings}
        \STATE $V_{\mathrm{HALO},n}=\{$node $v \in \mathcal{G}_n:v \notin V_n\}$ \COMMENT{Create HALO node set}
        \STATE Distribute $V_{\mathrm{HALO},n}$ and receive $[V_{\mathrm{HALO},1}, ..., V_{\mathrm{HALO},N}]$
        \STATE Distribute $V_n$ and receive $[V_{1}, ..., V_{N}]$
        \STATE $[S_1,...,S_N]=[V_n\cap V_{\mathrm{HALO},1}, ..., V_n\cap V_{\mathrm{HALO},N}]$ \COMMENT{Nodes to be sent}
        \STATE $[R_1,...,R_N]=[V_{\mathrm{HALO},n}\cap V_1,...,V_{\mathrm{HALO},n}\cap V_N]$ \COMMENT{Nodes to receive}

        \FOR{$t$ \textbf{from} $1$ \textbf{to} $T$ }
        \FOR{$l$ \textbf{from} $1$ \textbf{to} $L$ }
        \IF {$t>1$}
        \STATE wait for $worker^{(l)}_{t-1}$ completes
        \STATE $\tilde{\boldsymbol{H}}^{(l-1)}_n=$ concatenate$(\boldsymbol{H}^{(l-1)}_n, \tilde{\boldsymbol{R}}^{(l-1)})$
        \ENDIF
        
        \STATE \textbf{with} $worker^{(l)}_{t}$ \COMMENT{Parallel communication and embedding update}
        \STATE \quad \ \ $\hat{\boldsymbol{S}}^{(l-1)}_{1bit}=$ quantize$([\boldsymbol{H}^{(l-1)}_n(S_1),...,\boldsymbol{H}^{(l-1)}_n(S_N)])$ \COMMENT{Quantize sent embeddings}
        \STATE \quad \ \ Send $\hat{\boldsymbol{S}}^{(l-1)}_{1bit}$ to partition $1,...,N$. Receive $\hat{\boldsymbol{R}}^{(l-1)}_{1bit}$ from partition $1,...,N$
        \STATE \quad \ \ $\tilde{\boldsymbol{R}}^{(l-1)}=$ dequantize$(\hat{\boldsymbol{R}}^{(l-1)}_{1bit})$ \COMMENT{Dequantize received embeddings}
        
        \IF {$l \neq L$}
        \STATE $\boldsymbol{H}^{(l)}_n=\sigma\left(\boldsymbol{A}^\top_n \tilde{\boldsymbol{H}}^{(l-1)}_n \boldsymbol{W}^{(l)}_{t-1}\right)$ \COMMENT{Update embeddings}
        \ELSE
        \STATE $\boldsymbol{H}^{(l)}_n=\boldsymbol{A}^\top_n \tilde{\boldsymbol{H}}^{(l-1)}_n \boldsymbol{W}^{(l)}_{t-1}$

        \ENDIF
        \ENDFOR
        \STATE $\mathcal{L}=Loss(softmax(\boldsymbol{H}^{(L)}_n), Y_n)$

        \ENDFOR
        
    \end{algorithmic}
    \vskip 0.2in
\end{algorithm}

\textbf{Backward Propogation}. Alg.\ref{pbw} shows the backward phase of \SysNameP, and $\circ$ denotes Hadamard product. Here \SysNameP pipelines \textit{1-bit Module}, feature gradient communication with the backward computation (line 8-18). In each layer, the backward computation starts in parallel with \textit{1-bit Module} and the communication of feature gradients. Similarly, gradient staleness is introduced due to the overlap. The transmitted feature gradients in current epoch are prepared in the buffer for the next epoch, leading to stale feature gradients.

\vskip 0.1in
\begin{algorithm}[ht]
    \caption{Backward phase of \SysNameP}
    \small
    \label{pbw} 
    \begin{algorithmic}[1]
        \STATE {\bfseries Input:} Partition id $n$, label $Y_n$, adjacency matrix $\boldsymbol{A}_n$, epoch number $T$, layer size $L$, local node set $V_n$, weights $\boldsymbol{W}^{(l-1)}$
        \STATE \textbf{Partition} $n=1,2,...,N$ in Parallel:
        \FOR{$t$ \textbf{from} $1$ \textbf{to} $T$ }
        \FOR{$l$ \textbf{from} $L$ \textbf{to} $1$ }
        \IF {$l=L$}
        \STATE $\boldsymbol{J}^{(L)}_n=\nabla_{\boldsymbol{H}^{(L)}_n} \mathcal{L}$
        \ENDIF

        \STATE $\boldsymbol{G}^{(l)}_n=\left[\boldsymbol{A}_n \tilde{\boldsymbol{H}}^{(l-1)}_n\right]^{\top}\left(\boldsymbol{J}^{(l)}_n \circ \sigma^{\prime}\left(\boldsymbol{A}_n \tilde{\boldsymbol{H}}^{(l-1)}_n \boldsymbol{W}^{(l)}_{t-1}\right)\right)$ \COMMENT{Compute weight gradients}

        \IF {$l>1$}
        
        \STATE $\boldsymbol{J}^{(l-1)}_n = \boldsymbol{A}_n^{\top}\left(\boldsymbol{J}^{(l)}_n \circ \sigma^{\prime}\left(\boldsymbol{A}_n \tilde{\boldsymbol{H}}^{(l-1)}_n \boldsymbol{W}^{(l)}_{t-1}\right)\right)\left[\boldsymbol{W}^{(l)}_{t-1}\right]^{\top}$ \COMMENT {Compute feature gradients}
        \IF {$t>1$}
        \STATE wait for $worker^{(l)}_{t-1}$ completes
        \STATE $\boldsymbol{J}^{(l-1)}_n=\boldsymbol{J}^{(l-1)}_n + \tilde{\boldsymbol{R}}^{(l-1)}$ \COMMENT{Integrate feature gradients}
        \ENDIF

        \STATE \textbf{with} $worker^{(l)}_{t}$ \COMMENT{Parallel communication and embedding update}
        \STATE \quad \ \ $\hat{\boldsymbol{S}}^{(l-1)}_{1bit}=$ quantize$([\boldsymbol{J}^{(l-1)}_n(R_1),...,\boldsymbol{J}^{(l-1)}_n(R_N)])$ \COMMENT{Quantize sent feature gradients}
        \STATE \quad \ \ Send $\hat{\boldsymbol{S}}^{(l-1)}_{1bit}$ to partition $1,...,N$. Receive $\hat{\boldsymbol{R}}^{(l-1)}_{1bit}$ from partition $1,...,N$
        \STATE \quad \ \ $\tilde{\boldsymbol{R}}^{(l-1)}=$ dequantize$(\hat{\boldsymbol{R}}^{(l-1)}_{1bit})$ \COMMENT{Dequantize received embeddings}
        
        \ENDIF

        \ENDFOR
        \STATE $\boldsymbol{G}=AllReduce(\boldsymbol{G_n})$ \COMMENT{Gradient synchronization}
        \STATE $\boldsymbol{W}_t = \boldsymbol{W}_{t-1}-\eta \boldsymbol{G}$ \COMMENT{Update model}

        \ENDFOR
        
    \end{algorithmic}
\end{algorithm}

%-------------------------------------------------------------------------------
\newpage
\section{Thoeretical Analysis}
\label{app_theory}

\subsection{Deduction of Theorem \ref{theorem1}}
\label{app_theorem1}
For quantized data $\boldsymbol{h}^{(l)}_{1bit}$ and dequantized data $\tilde{\boldsymbol{h}}^{(l)}$, we have the following conclusions
\begin{align}
    \mathbb{E}\left[\tilde{\boldsymbol{h}}^{(l)}\right]&=\mathbb{E}[\mathrm{Dequantize}(\mathrm{Quantize}(\boldsymbol{h}^{(l)}))]=\boldsymbol{h}^{(l)}  \\ 
    \mathrm{Var}(\tilde{\boldsymbol{h}}^{(l)})&=\frac{D\left[ \max(\boldsymbol{h}^{(l)})-\min(\boldsymbol{h}^{(l)})\right]^2}{6 B^2} 
\end{align}

These conclusions are referenced from ActNN \citep{ActNN} and the deduction of them is referenced from EXACT \citep{EXACT}. Those conclusions are successfully drawn under the unbiased nature of stochastic rounding \citep{BinaryConnect} presented in Equ.\ref{rounding}, where $\lceil\cdot\rceil$ is the ceiling function and $\lfloor\cdot\rfloor$ is the floor function. We can derive $\mathbb{E}[\lfloor \boldsymbol{h}^{(l)} \rceil]=\boldsymbol{h}^{(l)}$ because 
\begin{align}
    \mathbb{E}[\lfloor x\rceil] &=\lceil x\rceil(x-\lfloor x\rfloor)+\lfloor x\rfloor(1-x+\lfloor x\rfloor) \notag \\ 
    &=x \notag
\end{align}

where $\lceil x\rceil-\lfloor x\rfloor=1$. Therefore, from Equ.\ref{quantize} and \ref{dequantize} we can further derive
$$
\begin{aligned}
\mathbb{E}\left[\tilde{\boldsymbol{h}}^{(l)}\right]&=\mathbb{E}\left[\mathrm{Dequantize}(\mathrm{Quantize}(\boldsymbol{h}^{(l)}))\right] \\
&=\frac{s^{(l)}}{B} \mathbb{E}\left[\left\lfloor\frac{\boldsymbol{h}^{(l)}-\min(\boldsymbol{h}^{(l)})}{s^{(l)}} B\right\rceil\right]+\min(\boldsymbol{h}^{(l)}) \\
&=\boldsymbol{h}^{(l)}
\end{aligned}
$$

where $s^{(l)}=\max(\boldsymbol{h}^{(l)})-\min(\boldsymbol{h}^{(l)})$. As for the variance of dequantized data, first we suppose $\bar{\boldsymbol{h}}^{(l)}=\left(h_{1}, \cdots, h_{D}\right)$, where $\bar{\boldsymbol{h}}^{(l)}$ is defined in Equ.\ref{quantize}. Suppose $\forall i \in [1,D], h_{i}-\left\lfloor h_{i}\right\rfloor=\sigma \sim$ Uniform $(0,1)$, we can derive
$$
\begin{aligned}
\operatorname{Var}\left(\tilde{\boldsymbol{h}}^{(l)}\right)
=\frac{\left[s^{(l)}\right]^{2}}{B^{2}} \operatorname{Var}(\lfloor\bar{\boldsymbol{h}}^{(l)}\rceil) 
&=\mathbb{E}\left[\bar{\boldsymbol{h}}^{\top} \bar{\boldsymbol{h}}\right]-(\mathbb{E}[\bar{\boldsymbol{h}}])^{\top}(\mathbb{E}[\bar{\boldsymbol{h}}]) \\
&=\frac{\left[s^{(l)}\right]^{2}}{B^{2}} \sum_{i=1}^{D}\left\lceil h_{i}\right\rceil^{2}\left(h_{i}-\left\lfloor h_{i}\right\rfloor\right)+\left\lfloor h_{i}\right\rfloor^{2}\left(1-h_{i}+\left\lfloor h_{i}\right\rfloor\right)-h_{i}^{2} \\
&=\frac{\left[s^{(l)}\right]^{2}D}{B^{2}}\left(2\left\lfloor h_{1}\right\rfloor h_{1}+h_{1}-\left\lfloor h_{1}\right\rfloor^{2}-\left\lfloor h_{1}\right\rfloor-h_{1}^{2}\right) \quad \text { (replace }\left\lceil h_{1}\right\rceil \text { with }\left\lfloor h_{1}\right\rfloor+1 \text { ) } \\
&=\frac{\left[s^{(l)}\right]^{2}D}{B^{2}}\left(\sigma-\sigma^{2}\right) \quad \text { (replace }\left\lfloor h_{1}\right\rfloor \text { with } h_{1}-\sigma \text { ) }
\end{aligned}
$$

Finally, we take expectation w.r.t. $\sigma$ on both sides, we have
\begin{align}
\mathrm{Var}(\tilde{\boldsymbol{h}}^{(l)})&=\frac{D\left[ s^{(l)}\right]^2}{6 B^2} \notag
\end{align}

This shows the strong bound of embeddings when applied extreme quantization.  

\subsection{Deduction of Theorem \ref{theorem2}}
\label{app_theorem2}
To prove the calculated gradients are unbiased, some parts of theories are adopted from \citet{ActNN}. Utilizing the quantization context $\hat{\mathbf{C}}$, the forward propagation(FP) gradients can be written as
$$
\hat{\boldsymbol{J}}^{(l-1)}, \hat{\boldsymbol{G}}^{(l)}=\mathbf{B}^{(l)}\left(\hat{\boldsymbol{J}}^{(l)}, \hat{\mathbf{C}}\left(\boldsymbol{H}^{(l-1)}, \boldsymbol{W}^{(l)}\right)\right)
$$

Assume the FP gradient is unbiased, we have $\mathbb{E}\left[\boldsymbol{G}^{(l)}\right]=\boldsymbol{G}^{(l)}$. If $\mathbb{E}\left[\hat{\boldsymbol{J}}^{(l)}\right]=\boldsymbol{J}^{(l)}$, according to the chain rule, the back propagation can be expressed as
$$
J^{(l-1)}_{ij}=\sum_{k l} \frac{\partial H_{k l}^{(l)}}{\partial H_{i j}^{(l-1)}} J^{(l)}_{kl}, \quad G^{(l)}_{i}=\sum_{k l} \frac{\partial H_{k l}^{(l)}}{\partial W_i^{(l)}} J^{(l)}_{kl}
$$

Therefore, we can write
$$
\mathbf{B}^{(l)}\left(\boldsymbol{J}^{(l)}, \mathbf{C}\left(\boldsymbol{H}^{(l-1)}, \boldsymbol{W}^{(l)}\right)\right)=\left\{\sum_{k l} \frac{\partial H_{k l}^{(l)}}{\partial H_{i j}^{(l-1)}} J^{(l)}_{kl}\right\}_{i j},\left\{\sum_{k l} \frac{\partial H_{k l}^{(l)}}{\partial W_i^{(l)}} J^{(l)}_{kl}\right\}_{i}
$$

where $\mathbf{C}\left(\boldsymbol{H}^{(l-1)}, \boldsymbol{W}^{(l)}\right)=\left\{\partial H_{k l}^{(l)} / \partial H_{i j}^{(l-1)}, \partial H_{k l}^{(l)} / \partial W_{i}^{(l)}\right\}_{i j k l}$. Let $\hat{\mathbf{C}}\left(\boldsymbol{H}^{(l-1)}, \boldsymbol{W}^{(l)}\right)=Q\left(\mathbf{C}\left(\boldsymbol{H}^{(l-1)}, \boldsymbol{W}^{(l)}\right)\right)$, where $Q(\cdot)$ is an unbiased quantization operation. Then we have
$$
\begin{aligned}
& \mathbb{E}\left[\hat{\boldsymbol{J}}^{(l-1)}, \hat{\boldsymbol{G}}^{(l)}\right]\\
=&\mathbb{E}\left[\mathbf{B}^{(l)}\left(\hat{\boldsymbol{J}}^{(l)}, \hat{\mathbf{C}}\left(\boldsymbol{H}^{(l-1)}, \boldsymbol{W}^{(l)}\right)\right)\right]\\
=&\mathbb{E}\left[\left\{\sum_{k l} Q\left(\frac{\partial H_{k l}^{(l)}}{\partial H_{i j}^{(l-1)}}\right) \hat{J}^{(l)}_{kl}\right\}_{i j},\left\{\sum_{k l} Q\left(\frac{\partial H_{k l}^{(l)}}{\partial W_{i}^{(l)}}\right) \hat{J}^{(l)}_{kl}\right\}_{i}\right] \\
=&\left\{\sum_{k l} \frac{\partial H_{k l}^{(l)}}{\partial H_{i j}^{(l-1)}} J^{(l)}_{kl}\right\}_{i j},\left\{\sum_{k l} \frac{\partial H_{k l}^{(l)}}{\partial W_{i}^{(l)}} J^{(l)}_{kl}\right\}_{i} \\
=& \mathbf{B}^{(l)}\left(\boldsymbol{J}^{(l)}, \mathbf{C}\left(\boldsymbol{H}^{(l-1)}, \boldsymbol{W}^{(l)}\right)\right)\\
=& \boldsymbol{J}^{(l-1)}, \boldsymbol{G}^{(l)} 
\end{aligned}
$$

Through this deduction, we can get $\mathbb{E}[\hat{\boldsymbol{J}}^{(l)}]=\mathbb{E}[\boldsymbol{J}^{(l)}]$, $\mathbb{E}[\hat{\boldsymbol{G}}^{(l)}]=\mathbb{E}[\boldsymbol{G}^{(l)}]$, $\forall$ $l \in \{1, \ldots, L\}$. And we already know $\mathbb{E}\left[\boldsymbol{G}^{(l)}\right]=\boldsymbol{G}^{(l)}$, so finally we can derive $\mathbb{E}[\hat{\boldsymbol{G}}^{(l)}]=\boldsymbol{G}^{(l)}$.

In the following we get the gradient variance (Equ.\ref{grad_variance}). According to the law of total variance
$$
\operatorname{Var}[X]=\mathbb{E}[\operatorname{Var}[X \mid Y]]+\operatorname{Var}[\mathbb{E}[X \mid Y]]
$$

First we have 
$$
\operatorname{Var}\left[\mathbf{B}_{\boldsymbol{W}}^{(l \sim L)}\left(\hat{\boldsymbol{J}}^{(L)}\right)\right]=\operatorname{Var}\left[\mathbf{B}_{\boldsymbol{W}}^{(l \sim L)}\left(\boldsymbol{J}^{(L)}\right)\right]=\operatorname{Var}\left[\boldsymbol{J}^{(L)}\right]
$$

For all $m<L$, by definition of $\hat{\boldsymbol{J}}^{(m)}$, we can get
$$
\operatorname{Var}\left[\mathbf{B}_{\boldsymbol{W}}^{(l \sim m)}\left(\hat{\boldsymbol{J}}^{(m)}\right)\right]=\operatorname{Var}\left[\mathbf{B}_{\boldsymbol{W}}^{(l \sim m)}\left(\mathbf{B}_{\boldsymbol{H}}^{(m+1)}\left(\hat{\boldsymbol{J}}^{(m+1)}, \hat{\mathbf{C}}^{(m+1)}\right)\right)\right]
$$

Using the law of total variance
$$
\operatorname{Var}\left[\mathbf{B}_{\boldsymbol{W}}^{(l \sim m)}\left(\hat{\boldsymbol{J}}^{(m)}\right)\right]=\operatorname{Var}\left[\boldsymbol{J}^{(l)}\right]+\sum_{j=m+1}^{L} \mathbb{E}\left[\operatorname{Var}\left[\mathbf{B}_{\boldsymbol{W}}^{(l \sim j)}\left(\hat{\boldsymbol{J}}^{(j)}, \hat{\mathbf{C}}^{(j)}\right) \mid \hat{\boldsymbol{J}}^{(j)}\right]\right]
$$

Then the variance of gradients
$$
\begin{aligned}
\operatorname{Var}\left[\hat{\boldsymbol{G}}^{(l)}\right]&=\operatorname{Var}\left[\mathbf{B}_{\boldsymbol{W}}^{(l)}\left(\hat{\nabla}_{\mathbf{H}^{(l)}}, \hat{\mathbf{C}}^{(l)}\right)\right] \\
&=\mathbb{E}\left[\operatorname{Var}\left[\mathbf{B}_{\boldsymbol{W}}^{(l)}\left(\hat{\boldsymbol{J}}^{(l)}, \hat{\mathbf{C}}^{(l)}\right) \mid \hat{\boldsymbol{J}}^{(l)}\right]\right]+\operatorname{Var}\left[\mathbb{E}\left[\mathbf{B}_{\boldsymbol{W}}^{(l)}\left(\hat{\boldsymbol{J}}^{(l)}, \hat{\mathbf{C}}^{(l)}\right) \mid \hat{\boldsymbol{J}}^{(l)}\right]\right] \\
&=\mathbb{E}\left[\operatorname{Var}\left[\mathbf{B}_{\boldsymbol{W}}^{(l \sim l)}\left(\hat{\boldsymbol{J}}^{(l)}, \hat{\mathbf{C}}^{(l)}\right) \mid \hat{\boldsymbol{J}}^{(l)}\right]\right]+\operatorname{Var}\left[\mathbf{B}_{\boldsymbol{W}}^{(l \sim l)}\left(\hat{\boldsymbol{J}}^{(l)}\right)\right] \\
&=\mathbb{E}\left[\operatorname{Var}\left[\mathbf{B}_{\boldsymbol{W}}^{(l \sim l)}\left(\hat{\boldsymbol{J}}^{(l)}, \hat{\mathbf{C}}^{(l)}\right) \mid \hat{\boldsymbol{J}}^{(l)}\right]\right]+\operatorname{Var}\left[\boldsymbol{J}^{(l)}\right]+\sum_{j=l+1}^L \mathbb{E}\left[\operatorname{Var}\left[\mathbf{B}_{\boldsymbol{W}}^{(l \sim j)}\left(\hat{\boldsymbol{J}}^{(l)}, \hat{\mathbf{C}}^{(j)}\right) \mid \hat{\boldsymbol{J}}^{(j)}\right]\right] \\
&=\mathrm{Var}\left[\boldsymbol{G}^{(l)}\right]+\sum_{m=l}^L \mathbb{E}\left[\mathrm{Var}\left[\mathbf{B}_{\boldsymbol{W}}^{(l \sim m)}\left(\hat{\boldsymbol{J}}^{(m)}, \hat{\mathbf{C}}^{(m)}\right) \mid \hat{\boldsymbol{J}}^{(m)}\right]\right] 
\end{aligned}
$$

From the above gradient variance, we can conclude two insights. First, it shows the amount of variance quantization technique introduces. We can clearly see the variances introduced by quantization contexts will accumulate along layers, so the noise is relatively small for shallow models. Most GNNs are usually less than four layers, making them more noise-tolerant, and this improves the maintenance of the model accuracy. Second, since we are using full-graph training, the extra variance introduced by quantization can be compensated.

%-------------------------------------------------------------------------------
\newpage
\section{Experiment Settings}
\label{app_experimentsetup}
% \subsection{Datasets and Models}
\textbf{Datasets}. We use four datasets in our evaluations: (1) Reddit, (2) Yelp, (3) Ogbn-products, (4) Amazon. The detailed information of the above datasets is shown in Table \ref{table_dataset_info}. Reddit predicts communities of online posts based on the posts' contents and users' comments. Yelp categorizes the types of business based on users' reviews and users' relationships. Ogbn-products classifies Amazon products according to customers' reviews. Amazon predicts product categories using their properties and relations between them.

\begin{table}[ht]
    \centering
    \caption{Detailed information of datasets used for evaluation.}
    \vskip 0.1in
    \resizebox{0.8\linewidth}{!}{
        \begin{tabular}{@{}crrcccc@{}}
            \toprule
            \textbf{Datasets} & \textbf{\# Nodes} & \textbf{\# Edges} & \textbf{Features Dim.} & \textbf{\# Classes} & \textbf{Train / Val / Test} & \textbf{Degree} \\ \midrule
            Reddit            & 232,965           & 114,615,892        & 602                    & 41                  & 0.66 / 0.10 / 0.24          & 492             \\
            Yelp              & 716,847           & 6,977,410         & 300                    & 100                 & 0.75 / 0.10 / 0.15          & 10             \\
            Ogbn-products     & 2,449,029         & 61,859,140        & 100                    & 47                  & 0.08 / 0.02 / 0.90          & 50.5           \\
            Amazon            & 1,598,960         & 132,169,734       & 200                    & 107                 & 0.85 / 0.05 / 0.10          & 83             \\ \bottomrule
            \end{tabular}
            }
    \label{table_dataset_info}
    \vskip 0.2in
\end{table}

\textbf{Model Structure}. Here we use three popular GNN models: (1) GraphSAGE, (2) GCN, (3) GAT: the number of heads are set to 1. Regarding the models, we follow the hyperparameter configurations reported in the corresponding papers as closely as possible. The detailed model hyperparameters used in our models in evaluation are presented in Table \ref{table_models_info}. GraphSAGE is a variant of GCN and pioneers in the use of node sampling to reduce the computational cost of aggregation. GCN is widely used for semi-supervised learning and uses spectral graph convolutions for aggregating the neighboring nodes. GAT uses the transformer approach in a learned attention mechanism to update node features.

\begin{table}[ht]
    \centering
    % \vspace{-20pt}
    \caption{Model structure and detailed hyperparameters used for evaluation.}
    \vskip 0.1in
    \resizebox{0.8\linewidth}{!}{
       \begin{tabular}{@{}ccccc|cccc@{}}
\toprule
\multicolumn{1}{l}{} & \multicolumn{4}{c|}{\textbf{\# Layers}}                                    & \multicolumn{4}{c}{\textbf{Hidden size}}                                   \\ \midrule
\textbf{Model}       & \textbf{Reddit} & \textbf{Yelp} & \textbf{Ogbn-products} & \textbf{Amazon} & \textbf{Reddit} & \textbf{Yelp} & \textbf{Ogbn-products} & \textbf{Amazon} \\ \midrule
GraphSAGE   & 4               & 4             & 3                      & 4               & 256             & 512           & 128                    & 512             \\
GCN         & 4               & 4             & 3                      & 4               & 256             & 512           & 128                    & 512             \\
GAT         & 2               & 2             & 3                      & 3               & 256             & 256           & 128                    & 128             \\ \bottomrule
\end{tabular}
            }
    \label{table_models_info}
    \vskip 0.2in
\end{table}

\textbf{Other configurations}. Other hyperparameter configurations in training are listed in Table \ref{table_hyperparameter}. The optimizer is Adam \cite{Adam} for all datasets and models. We use the default hyperparameters for Adam optimizer, except for the learning rate. All methods terminate after a fixed number of epochs. We report the test accuracy/F1-micro score associated with the highest validation score. 

\begin{table}[ht]
    \centering
    % \vspace{-20pt}
    \caption{Training hyperparameters used for evaluation.}
    \vskip 0.1in
    \resizebox{0.65\linewidth}{!}{
      \begin{tabular}{@{}cccccc@{}}
\toprule
\textbf{Model}             & \multicolumn{1}{l}{\textbf{Training Parameter}} & \textbf{Reddit} & \textbf{Yelp} & \textbf{Ogbn-products} & \textbf{Amazon} \\ \midrule
\multirow{3}{*}{GraphSAGE} & Learning Rate                                   & 0.01            & 0.01          & 0.01                   & 0.01            \\
                           & Epochs                                          & 2000            & 2000          & 500                    & 2000            \\
                           & Dropout                                         & 0.5             & 0.1           & 0.3                    & 0.1             \\ \midrule
\multirow{3}{*}{GCN}       & Learning Rate                                   & 0.01            & 0.01          & 0.01                   & 0.01            \\
                           & Epochs                                          & 2000            & 2000          & 500                    & 2000            \\
                           & Dropout                                         & 0.5             & 0.1           & 0.3                    & 0.1             \\ \midrule
\multirow{3}{*}{GAT}       & Learning Rate                                   & 0.01            & 0.01          & 0.01                   & 0.01            \\
                           & Epochs                                          & 200             & 1000          & 200                    & 1000            \\
                           & Dropout                                         & 0.5             & 0.1           & 0.3                    & 0.1             \\ \bottomrule
\end{tabular}
            }
    \label{table_hyperparameter}
    \vskip 0.2in
\end{table}

%-------------------------------------------------------------------------------
\newpage
\section{Full Results over Single Server}
\label{app_singlenode}
%-------------------------------------------------------------------------------

The full results of training throughput over single server are presented in Table \ref{table_single_node}. Apparently, the performance of \SysName also exceeds all SOTA baselines on all datasets by up to 9.31$\times$ compared with DGL. Though for GAT on Amazon dataset, the throughput achieved by PipeGCN (1.40$\times$) is slightly better than that of \SysNameS(1.37$\times$), \SysNameP still offers the best throughput(1.42$\times$) than other methods. By pipelining \textit{1-bit Module} and computation, \SysNameP further facilitates the training efficiency on the base of \SysNameS.

\begin{table}[ht]
    \centering
    % \vspace{-20pt}
    \caption{Normalized training throughput between our methods and baselines when training over single-server, where the best performance is highlighted.}
    \vskip 0.1in
    \resizebox{0.9\linewidth}{!}{
        \begin{tabular}{@{}cccccc@{}}
            \toprule
            \multirow{2}{*}{\textbf{Model}}                                                          & \multirow{2}{*}{\textbf{Method}} & \textbf{Reddit}             & \textbf{Yelp}               & \textbf{Ogbn-products}      & \textbf{Amazon}             \\ \cmidrule(l){3-6} 
                                                                                                     &                                  & \textbf{Thr.}               & \textbf{Thr.}               & \textbf{Thr.}               & \textbf{Thr.}               \\ \midrule
            \multirow{6}{*}{\textbf{\begin{tabular}[c]{@{}c@{}}GraphSAGE\\      (N=4)\end{tabular}}} & DGL                              & 1.00$\times$(2.23 epochs/s) & 1.00$\times$(2.25 epochs/s) & 1.00$\times$(1.22 epochs/s) & 1.00$\times$(0.55 epochs/s) \\
                                                                                                     & SAR                              & 0.58$\times$                & 0.99$\times$                & 1.27$\times$                & 1.11$\times$                \\
                                                                                                     & PipeGCN                          & 1.16$\times$                & 1.26$\times$                & 1.18$\times$                & 1.10$\times$                \\
                                                                                                     & BNS-GCN                          & 3.00$\times$                & 2.95$\times$                & 2.09$\times$                & 2.64$\times$                \\
                                                                                                     & 1BG-S                            & 3.85$\times$                & 3.83$\times$                & 2.76$\times$                & 2.93$\times$                \\
                                                                                                     & 1BG-A                            & \textbf{4.89}$\times$       & \textbf{4.48}$\times$       & \textbf{3.68}$\times$       & \textbf{3.32}$\times$       \\ \cmidrule(l){2-6} 
            \multirow{6}{*}{\textbf{\begin{tabular}[c]{@{}c@{}}GraphSAGE\\      (N=8)\end{tabular}}} & DGL                              & 1.00$\times$(1.51 epochs/s) & 1.00$\times$(1.82 epochs/s) & 1.00$\times$(0.95 epochs/s) & 1.00$\times$(0.38 epochs/s) \\
                                                                                                     & SAR                              & 0.56$\times$                & 0.99$\times$                & 1.27$\times$                & 1.12$\times$                \\
                                                                                                     & PipeGCN                          & 1.06$\times$                & 1.08$\times$                & 1.05$\times$                & 0.97$\times$                \\
                                                                                                     & BNS-GCN                          & 3.35$\times$                & 3.10$\times$                & 3.07$\times$                & 6.93$\times$                \\
                                                                                                     & 1BG-S                            & 5.71$\times$                & 5.49$\times$                & 4.71$\times$                & 7.71$\times$                \\
                                                                                                     & 1BG-A                            & \textbf{7.24}$\times$       & \textbf{6.38}$\times$       & \textbf{6.98}$\times$       & \textbf{9.31}$\times$       \\ \midrule
            \multirow{6}{*}{\textbf{\begin{tabular}[c]{@{}c@{}}GCN\\      (N=4)\end{tabular}}}       & DGL                              & 1.00$\times$(2.65 epochs/s) & 1.00$\times$(2.30 epochs/s) & 1.00$\times$(1.35 epochs/s) & 1.00$\times$(0.59 epochs/s) \\
                                                                                                     & SAR                              & 0.59$\times$                & 1.06$\times$                & 1.33$\times$                & 1.25$\times$                \\
                                                                                                     & PipeGCN                          & 1.13$\times$                & 1.20$\times$                & 1.21$\times$                & 1.05$\times$                \\
                                                                                                     & BNS-GCN                          & 2.82$\times$                & 2.58$\times$                & 1.76$\times$                & 2.22$\times$                \\
                                                                                                     & 1BG-S                            & 3.45$\times$                & 3.56$\times$                & 2.63$\times$                & 2.58$\times$                \\
                                                                                                     & 1BG-A                            & \textbf{4.23}$\times$       & \textbf{4.26}$\times$       & \textbf{3.50}$\times$       & \textbf{2.83}$\times$       \\ \cmidrule(l){2-6} 
            \multirow{6}{*}{\textbf{\begin{tabular}[c]{@{}c@{}}GCN\\      (N=8)\end{tabular}}}       & DGL                              & 1.00$\times$(1.89 epochs/s) & 1.00$\times$(1.91 epochs/s) & 1.00$\times$(1.12 epochs/s) & 1.00$\times$(0.42 epochs/s) \\
                                                                                                     & SAR                              & 0.57$\times$                & 1.04$\times$                & 1.32$\times$                & 1.23$\times$                \\
                                                                                                     & PipeGCN                          & 1.03$\times$                & 1.07$\times$                & 1.06$\times$                & 0.94$\times$                \\
                                                                                                     & BNS-GCN                          & 3.10$\times$                & 2.30$\times$                & 2.46$\times$                & 4.78$\times$                \\
                                                                                                     & 1BG-S                            & 4.93$\times$                & 5.50$\times$                & 3.51$\times$                & 6.06$\times$                \\
                                                                                                     & 1BG-A                            & \textbf{6.41}$\times$       & \textbf{6.93}$\times$       & \textbf{5.46}$\times$       & \textbf{8.00}$\times$       \\ \midrule
            \multirow{6}{*}{\textbf{\begin{tabular}[c]{@{}c@{}}GAT\\      (N=4)\end{tabular}}}       & DGL                              & 1.00$\times$(5.87 epochs/s) & 1.00$\times$(4.94 epochs/s) & 1.00$\times$(1.31 epochs/s) & 1.00$\times$(0.95 epochs/s) \\
                                                                                                     & SAR                              & 0.11$\times$                & 0.097$\times$               & 0.26$\times$                & 0.40$\times$                \\
                                                                                                     & PipeGCN                          & 1.58$\times$                & 1.33$\times$                & 1.50$\times$                & 1.40$\times$                \\
                                                                                                     & BNS-GCN                          & 1.65$\times$                & 2.83$\times$                & 1.64$\times$                & 1.21$\times$                \\
                                                                                                     & 1BG-S                            & 1.99$\times$                & 3.18$\times$                & 1.91$\times$                & 1.37$\times$                \\
                                                                                                     & 1BG-A                            & \textbf{2.10}$\times$       & \textbf{3.52}$\times$       & \textbf{2.01}$\times$       & \textbf{1.42}$\times$       \\ \cmidrule(l){2-6} 
            \multirow{6}{*}{\textbf{\begin{tabular}[c]{@{}c@{}}GAT\\      (N=8)\end{tabular}}}       & DGL                              & 1.00$\times$(4.73 epochs/s) & 1.00$\times$(4.00 epochs/s) & 1.00$\times$(1.24 epochs/s) & 1.00$\times$(0.84 epochs/s) \\
                                                                                                     & SAR                              & 0.10$\times$                & 0.10$\times$                & 0.25$\times$                & 0.30$\times$                \\
                                                                                                     & PipeGCN                          & 1.19$\times$                & 1.14$\times$                & 1.02$\times$                & 1.17$\times$                \\
                                                                                                     & BNS-GCN                          & 2.51$\times$                & 2.87$\times$                & 2.49$\times$                & 2.80$\times$                \\
                                                                                                     & 1BG-S                            & 2.83$\times$                & 4.55$\times$                & 3.23$\times$                & 2.88$\times$                \\
                                                                                                     & 1BG-A                            & \textbf{3.05}$\times$       & \textbf{5.56}$\times$       & \textbf{3.46}$\times$       & \textbf{3.06}$\times$       \\ \bottomrule
            \end{tabular}
            }
    \label{table_single_node}
    \vskip 0.2in
\end{table}

% Why reduce time increase/reduce? AllReduce overhead may be caused by imbalance computation. Some partitions with low workload have to wait for other slow partitions, and the waiting time may dominate AllReduce overhead.
